# Supplementary material for: Strain-driven chiral phonons in two-dimensional hexagonal materials
Source: arXiv:2201.04909 ancillary file (2022-01-13)
Supplement: Supplementary file 1 [file SM_final.pdf]

# Supplemental Material: "Strain-driven chiral phonons in two-dimensional hexagonal materials"

Habib Rostami,[1] Francisco Guinea,[2, 3, 4] and Emmanuele Cappelluti[5]

[1]*Nordita, KTH Royal Institute of Technology and Stockholm University, Hannes Alfvéns väg 12, 10691 Stockholm, Sweden*

[2]*Imdea Nanoscience, Faraday 9, 28047 Madrid, Spain*

[3]*Donostia International Physics Center, Paseo Manuel de Lardizábal 4, 20018 San Sebastián, Spain*

[4]*Ikerbasque. Basque Foundation for Science. 48009 Bilbao. Spain.*

[5]*Istituto di Struttura della Materia-CNR (ISM-CNR), Trieste, Italy*

(Dated: January 13, 2022)

## CONTENTS

S1. Dynamical matrix by means of force-constant models 1

S2. Strain effects on dynamical matrix in hexagonal lattices 3

S3. Effective models for optical phonon around Γ-point 4

References 5

## S1. DYNAMICAL MATRIX BY MEANS OF FORCE-CONSTANT MODELS

In this Section we detail the microscopical calculation employed to evaluate in the paper the dynamical matrix, and hence the phonon dispersion and the phonon eigenvector.

We employ a force-constant (FC) model on a bipartite hexagonal lattice with two different masses $M_\alpha$, with $\alpha = 1, 2$. We set the armchair direction along the $x$-axis and we denote as atom 1 the atom on the left of the $x$-axis bond (see Fig. 1a of the main text). Given the inter-atomic distance $a$, for the atom 1 we have thus three nearest neighbors at

$$\boldsymbol{\delta}_1^{(0)} = a(1, 0), \tag{S1}$$

$$\boldsymbol{\delta}_2^{(0)} = a(-1/2, \sqrt{3}/2), \tag{S2}$$

$$\boldsymbol{\delta}_3^{(0)} = a(-1/2, -\sqrt{3}/2). \tag{S3}$$

Following Ref. S1 and S2, we consider elastic forces only between nearest neighbors. We define the vector of the lattice displacements for the unit cell $i$ in real space as:

$$\mathbf{u}_i = \begin{pmatrix} u_{1,x}(\mathbf{r}_i) \\ u_{1,y}(\mathbf{r}_i) \\ u_{2,x}(\mathbf{r}_i) \\ u_{2,y}(\mathbf{r}_i) \end{pmatrix}, \tag{S4}$$

and in the momentum space:

$$\mathbf{u}_\mathbf{q} = \begin{pmatrix} u_{1,x}(\mathbf{q}) \\ u_{1,y}(\mathbf{q}) \\ u_{2,x}(\mathbf{q}) \\ u_{2,y}(\mathbf{q}) \end{pmatrix}. \tag{S5}$$

We consider as a representative case the simplest spring-model containing one radial ($\phi_r$) and one transverse ($\phi_t$) force constant acting between nearest neighbor atoms (see Figure S1). According, it is convenient to define in the cartesian $x - y$ space the stiffness matrix along the bond 1as:

$$\boldsymbol{\Phi}_1 = \begin{pmatrix} \phi_r & 0 \\ 0 & \phi_t \end{pmatrix}. \tag{S6}$$

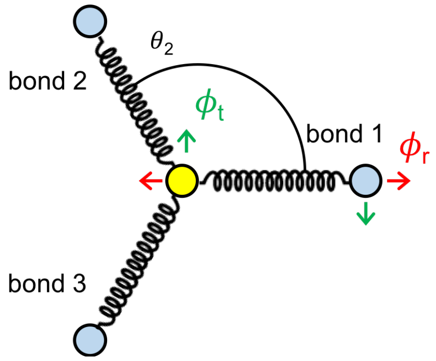


FIG. S1. Sketch of the relevant geometry and force-constant parameters employed in the present modelling. Yellow balls represent atoms on the sublattice 1, light blue balls atoms on the sublattice 2. Each atom on the sublattice 1 is connected to three nearest neightbor atoms on the sublattice 2 through three geometrically different bonds. The force-constant $\phi_r$ rules the elastic properties of the lattice displacement along the bond direction, $\phi_t$ the elastic properties of the lattice displacement perpendicular to the bond direction. Als shown is the definition of the $\theta$ angle between nearest neighbor atoms, here depicted for bond 2.

In similar way, the stiffness matrix operative for bond 2 and 3 can be obtain just with a rotation matrix by $\pm\theta = \pm 2\pi/3$, namely:

$$\mathbf{\Phi}_2 = U^{-1}(\theta)\mathbf{\Phi}_1 U(\theta) = \frac{1}{4}\begin{pmatrix} \phi_r + 3\phi_t & -\sqrt{3}(\phi_r - \phi_t) \\ -\sqrt{3}(\phi_r - \phi_t) & 3\phi_r + \phi_t \end{pmatrix}, \tag{S7}$$

and

$$\mathbf{\Phi}_3 = U^{-1}(-\theta)\mathbf{\Phi}_1 U(-\theta) = \frac{1}{4}\begin{pmatrix} \phi_r + 3\phi_t & \sqrt{3}(\phi_r - \phi_t) \\ \sqrt{3}(\phi_r - \phi_t) & 3\phi_r + \phi_t \end{pmatrix}, \tag{S8}$$

where

$$U(\theta) = \begin{pmatrix} \cos\theta & \sin\theta \\ -\sin\theta & \cos\theta \end{pmatrix} = \begin{pmatrix} -1/2 & \sqrt{3}/2 \\ -\sqrt{3}/2 & -1/2 \end{pmatrix}. \tag{S9}$$

The equation of motion for the lattice displacement along each direction and for each atom reads thus:

$$\hat{\mathbf{M}} \cdot \left(\frac{\partial^2 \mathbf{u}_i}{\partial t^2}\right) = -\sum_{\langle j\rangle_i} \hat{\mathbf{K}}_{i-j} \cdot \mathbf{u}_j, \tag{S10}$$

where $\langle j\rangle_i$ denotes sites $j$ nearest neighbors of the site $i$, $\hat{\mathbf{M}}$ is a diagonal matrix:

$$\hat{\mathbf{M}} = \begin{pmatrix} M_1 & 0 & 0 & 0 \\ 0 & M_1 & 0 & 0 \\ 0 & 0 & M_2 & 0 \\ 0 & 0 & 0 & M_2 \end{pmatrix}, \tag{S11}$$

and $\hat{\mathbf{K}}_{i-j}$ is the matrix of the elastic constants in the real space. Eq. (S10) can be equivalently written in the momentum space:

$$\hat{\mathbf{M}} \cdot \left(\frac{\partial^2 \mathbf{u}_{\mathbf{q}}}{\partial t^2}\right) = -\hat{\mathbf{K}}_{\mathbf{q}} \cdot \mathbf{u}_{\mathbf{q}}. \tag{S12}$$

With the help of Eqs. (S6)-(S8), we can finally get an analytical expression for $\hat{\mathbf{K}}_{\mathbf{q}}$:

$$\hat{\mathbf{K}}_{\mathbf{q}} = \sum_{i=1}^{3} \begin{pmatrix} \mathbf{\Phi}_i & -\mathbf{\Phi}_i e^{i\mathbf{q}\cdot\boldsymbol{\delta}_i^{(0)}} \\ -\mathbf{\Phi}_i e^{-i\mathbf{q}\cdot\boldsymbol{\delta}_i^{(0)}} & \mathbf{\Phi}_i \end{pmatrix}. \tag{S13}$$

For practical purposes, it is more convenient to introduce the dynamical matrix $\hat{\mathbf{D}}_{\mathbf{q}}$ defined as:

$$\hat{\mathbf{D}}_{\mathbf{q}} = \hat{\mathbf{M}}^{-1/2} \cdot \hat{\mathbf{K}}_{\mathbf{q}} \cdot \hat{\mathbf{M}}^{-1/2}, \tag{S14}$$

and in the frequency space we get the (diagonal) matrix of the phonon dispersion $\boldsymbol{\omega}_{\mathbf{q}}$ (and the corresponding egigenvectors) from the solution:

$$\hat{\mathbf{D}}_{\mathbf{q}} \cdot \mathbf{u}_{\mathbf{q}} = \boldsymbol{\omega}_{\mathbf{q}}^2 \cdot \mathbf{u}_{\mathbf{q}}. \tag{S15}$$

## S2. STRAIN EFFECTS ON DYNAMICAL MATRIX IN HEXAGONAL LATTICES

In the present Section we generalize the nearest-neighbor force-constant model, previously introduced for a perfect hexagonal lattice, in the case of strain. The nearest neighbour vectors are modified by applying strain as:

$$\boldsymbol{\delta}_i = (1 + \boldsymbol{\varepsilon}) \cdot \boldsymbol{\delta}_i^{(0)} \tag{S16}$$

where $\boldsymbol{\delta}_i^{(0)}$ are the vectors of the nearest neighbors in the perfect hexagonal structure defined in Eqs. (S1)-(S3), and where the strain tensor is given by

$$\boldsymbol{\varepsilon} = \begin{pmatrix} \varepsilon_{xx} & \varepsilon_{xy} \\ \varepsilon_{xy} & \varepsilon_{yy} \end{pmatrix} \tag{S17}$$

Therefore, we find

$$\boldsymbol{\delta}_1 = a(1 + \varepsilon_{xx}, \varepsilon_{xy}) \tag{S18}$$

$$\boldsymbol{\delta}_2 = \frac{a}{2}(-1 - \varepsilon_{xx} + \sqrt{3}\varepsilon_{xy}, \sqrt{3}(1 + \varepsilon_{yy}) - \varepsilon_{xy}) \tag{S19}$$

$$\boldsymbol{\delta}_3 = \frac{a}{2}(-1 - \varepsilon_{xx} - \sqrt{3}\varepsilon_{xy}, -\sqrt{3}(1 + \varepsilon_{yy}) - \varepsilon_{xy}) \tag{S20}$$

In the presence of strain, the stiffness matrices in Eqs. (S6)-(S8) need to be adjusted to account for two different effects. On one hand, there is a “geometrical” effect, driven by the change of the angle in the cartesian space between the two bound atoms according the relation

$$\tan\theta_i = \delta_{i,y}/\delta_{i,x}. \tag{S21}$$

The rotation matrices for each bond is thus generalized as:

$$\mathbf{R}(\theta_i) = \begin{pmatrix} \cos\theta_i & \sin\theta_i \\ -\sin\theta_i & \cos\theta_i \end{pmatrix}, \tag{S22}$$

resulting in

$$\mathbf{R}(\theta_1) = \begin{pmatrix} 1 & \varepsilon_{xy} \\ -\varepsilon_{xy} & 1 \end{pmatrix}, \tag{S23}$$

$$\mathbf{R}(\theta_2) = \frac{1}{8}\begin{pmatrix} -3\varepsilon_{yy} + 2\sqrt{3}\varepsilon_{xy} + 3\varepsilon_{yy} - 4 & -\sqrt{3}\varepsilon_{xx} + 2\varepsilon_{xy} + \sqrt{3}(\varepsilon_{yy} + 4) \\ \sqrt{3}\varepsilon_{xx} - 2\varepsilon_{xy} - \sqrt{3}(\varepsilon_{yy} + 4) & -3\varepsilon_{xx} + 2\sqrt{3}\varepsilon_{xy} + 3\varepsilon_{xy} - 4 \end{pmatrix}, \tag{S24}$$

$$\mathbf{R}(\theta_3) = \frac{1}{8}\begin{pmatrix} -3\varepsilon_{xy} - 2\sqrt{3}\varepsilon_{xy} + 3\varepsilon_{yy} - 4 & \sqrt{3}\varepsilon_{xx} + 2\varepsilon_{xy} - \sqrt{3}(\varepsilon_{yy} + 4) \\ -\sqrt{3}\varepsilon_{xx} - 2\varepsilon_{xy} + \sqrt{3}(\varepsilon_{yy} + 4) & -3\varepsilon_{yy} - 2\sqrt{3}\varepsilon_{xx} + 3\varepsilon_{yy} - 4 \end{pmatrix}. \tag{S25}$$

Note that this effect is not present in the case of biaxial strain that preserves the perfect hexagonal symmetry. On the other hand, the strength of the spring constants $\phi_r(R)$, $\phi_t(R)$ depends itself on the interatomic distance $R$ which in the presence of strain is also changed. The strengths in the presence of strain $\bar{\phi}^i_{r,t}$ for each bond $i$ can be thus computed as

$$\phi^\varepsilon_{i,\ell} = \phi_\ell\left[1 - \frac{\beta_\ell}{a^2}\boldsymbol{\delta}_i^{(0)} \cdot \boldsymbol{\varepsilon} \cdot \boldsymbol{\delta}_i^{(0)}\right], \tag{S26}$$

where $\beta_{\ell=r,t} = -\partial\ln\phi_\ell/\partial\ln(a)$. Taking into account both effects leads to the relations:

$$\hat{\boldsymbol{\Phi}}^\varepsilon_1 = \begin{pmatrix} \phi^\varepsilon_{1,r} & g_1(\phi^\varepsilon_{1,r} - \phi^\varepsilon_{1,t}) \\ g_1(\phi^\varepsilon_{1,r} - \phi^\varepsilon_{1,t}) & \phi^\varepsilon_{1,t} \end{pmatrix}, \tag{S27}$$

$$\hat{\boldsymbol{\Phi}}^\varepsilon_2 = \begin{pmatrix} \phi^\varepsilon_{2,r}g_2 + \phi^\varepsilon_{2,t}g_3 & -(\phi^\varepsilon_{2,r} - \phi^\varepsilon_{2,t})g_4 \\ -(\phi^\varepsilon_{2,r} - \phi^\varepsilon_{2,t})g_4 & \phi^\varepsilon_{2,t}g_2 + \phi^\varepsilon_{2,r}g_3 \end{pmatrix}, \tag{S28}$$

$$\hat{\boldsymbol{\Phi}}^\varepsilon_3 = \begin{pmatrix} \phi^\varepsilon_{3,r}g_2 + \phi^\varepsilon_{3,t}g_3 & (\phi^\varepsilon_{3,r} - \phi^\varepsilon_{3,t})g_4 \\ (\phi^\varepsilon_{3,r} - \phi^\varepsilon_{3,t})g_4 & \phi^\varepsilon_{3,t}g_2 + \phi^\varepsilon_{3,r}g_3 \end{pmatrix}, \tag{S29}$$

where

$$\phi^{\varepsilon}_{1,\ell} = \phi_\ell \left\{1 - \beta_\ell \varepsilon_{xx}\right\} \tag{S30}$$

$$\phi^{\varepsilon}_{2,\ell} = \phi_\ell \left\{1 - \beta_\ell \frac{1}{4}(\varepsilon_{xx} - 2\sqrt{3}\varepsilon_{xy} + 3\varepsilon_{yy})\right\} \tag{S31}$$

$$\phi^{\varepsilon}_{3,\ell} = \phi_\ell \left\{1 - \beta_\ell \frac{1}{4}(\varepsilon_{xx} + 2\sqrt{3}\varepsilon_{xy} + 3\varepsilon_{yy})\right\}, \tag{S32}$$

and where

$$g_1 = \varepsilon_{xy}, \tag{S33}$$

$$g_2 = \frac{2 + 3(\varepsilon_{xx} - \varepsilon_{yy}) - 2\sqrt{3}\varepsilon_{xy}}{8}, \tag{S34}$$

$$g_3 = \frac{6 - 3(\varepsilon_{xx} - \varepsilon_{yy}) + 2\sqrt{3}\varepsilon_{xy}}{8}, \tag{S35}$$

$$g_4 = \frac{2\sqrt{3} + \sqrt{3}(\varepsilon_{xx} - \varepsilon_{yy}) - 2\varepsilon_{xy}}{8}. \tag{S36}$$

Eqs. (S27)-(S32), once plugged in Eq. (S13), define the matrix of the elastic constant $\hat{\mathbf{K}}^{\varepsilon}_{\mathbf{q}}$, and hence the dynamical matrix $\hat{\mathbf{D}}^{\varepsilon}_{\mathbf{q}}$, in the presence of strain, taking into account both the "geometrical" effects and the changes in the spring strengths.

## S3. EFFECTIVE MODELS FOR OPTICAL PHONON AROUND Γ-POINT

In this Section we employ a Schrieffer-Wolf transformation in order to obtain an effective model for optical modes near Γ point. From pratical purpose, we perform the derivation in the Cartesian space, whereas the equivalent expression in the chiral basis can be eventually obtained by a final rotation. We start our analysis by defining the dynamical matrix of the full lattice model at Γ point ($\mathbf{q} = \mathbf{0}$):

$$\hat{\mathbf{D}}_\Gamma = \sum_{i=1}^{3} \begin{pmatrix} \hat{\mathbf{\Phi}}_i/M_1 & -\hat{\mathbf{\Phi}}_i/\sqrt{M_1 M_2} \\ -\hat{\mathbf{\Phi}}_i/\sqrt{M_1 M_2} & \hat{\mathbf{\Phi}}_i/M_2 \end{pmatrix}. \tag{S37}$$

Such matrix can be diagonalized by the unitary transformation $\hat{\mathbf{U}}_\Gamma$:

$$\hat{\mathbf{D}}'_\Gamma = \hat{\mathbf{U}}_\Gamma \hat{\mathbf{D}}_\Gamma \hat{\mathbf{U}}_\Gamma^{-1}. \tag{S38}$$

It is straightforward to notice that:

$$\hat{\mathbf{D}}'_\Gamma = \begin{pmatrix} \omega_\Gamma^2 \hat{\mathrm{I}}_{2\times 2} & \hat{0}_{2\times 2} \\ \hat{0}_{2\times 2} & \hat{0}_{2\times 2} \end{pmatrix}, \tag{S39}$$

where $\hat{\mathrm{I}}_{2\times 2}$, $\hat{0}_{2\times 2}$ are the identity matrix and the null matrxi, respectively, in the $2 \times 2$ space. The unitary transformation $\hat{\mathbf{U}}_\Gamma$ can be used to express in such new basis the full lattice dynamical matrix:

$$\hat{\mathbf{D}}'_{\mathbf{q}} = \hat{\mathbf{U}}_\Gamma \hat{\mathbf{D}}_{\mathbf{q}} \hat{\mathbf{U}}_\Gamma^{-1}. \tag{S40}$$

In full generality, $\hat{\mathbf{D}}'_{\mathbf{q}}$ can be decomposed as:

$$\hat{\mathbf{D}}'_{\mathbf{q}} = \hat{\mathbf{D}}'_{0,\mathbf{q}} + \hat{\mathbf{V}}_{\mathbf{q}}, \tag{S41}$$

where $\hat{\mathbf{D}}'_{0,\mathbf{q}}$ is block diagonal with respect to the sub-spaces of optical and acoustic modes,

$$\hat{\mathbf{D}}'_{0,\mathbf{q}} = \begin{pmatrix} \hat{\mathbf{D}}'_{\mathrm{d,op}} & 0 \\ 0 & \hat{\mathbf{D}}'_{\mathbf{q},\mathrm{ac}} \end{pmatrix}, \tag{S42}$$

whereas $\hat{\mathbf{V}}_{\mathbf{q}}$ if "off-diagonal" and it accounts for the finite hybridization between these two blocks,

$$\hat{\mathbf{V}}_{\mathbf{q}} = \begin{pmatrix} 0 & \hat{\mathbf{V}}_{\mathbf{q},\mathrm{op-ac}} \\ \hat{\mathbf{V}}^\dagger_{\mathbf{q},\mathrm{op-ac}} & 0 \end{pmatrix}. \tag{S43}$$

By construction, it is easy to see that $\hat{\mathbf{V}}_{\mathbf{q}} \to 0$ for $|\mathbf{q}| \to 0$. Our aim is to obtain an effective model valid at the $q^2$ order for the two-band subset of the optical modes. Within this framework we can expand matrix elements in Eq. (S42) up to the $q^2$ order, and $\hat{\mathbf{V}}_{\mathbf{q}}$ up to the linear order. In order to derive an effective model, we perform thus a Schrieffer-Wolf transformation:

$$\hat{\mathbf{D}}''_{\mathbf{q}} = = e^{-\hat{\mathcal{S}}_{\mathbf{q}}}\hat{\mathbf{D}}'_{\mathbf{q}}e^{\hat{\mathcal{S}}_{\mathbf{q}}} \approx \hat{\mathbf{D}}'_{\mathbf{q}} + \hat{\mathbf{V}}_{\mathbf{q}} + \left[\hat{\mathbf{D}}'_{\mathbf{q}}, \hat{\mathcal{S}}_{\mathbf{q}}\right] + \left[\hat{\mathbf{V}}_{\mathbf{q}}, \hat{\mathcal{S}}_{\mathbf{q}}\right] + \frac{1}{2}\left[\left[\hat{\mathbf{D}}'_{\mathbf{q}}, \hat{\mathcal{S}}_{\mathbf{q}}\right], \hat{\mathcal{S}}_{\mathbf{q}}\right] + \text{higher order terms}, \quad \text{(S44)}$$

where $\hat{\mathcal{S}}_{\mathbf{q}}$ has an off-diagonal form:

$$\hat{\mathcal{S}}_{\mathbf{q}} = \begin{pmatrix} \hat{0}_{2\times 2} & \hat{\eta}_{\mathbf{q}} \\ -\hat{\eta}^\dagger_{\mathbf{q}} & \hat{0}_{2\times 2} \end{pmatrix}, \quad \text{(S45)}$$

where the $2 \times 2$ matrix can be identify by imposing the condition of cancellation of the $q$-linear terms:

$$\hat{\mathbf{V}}_{\mathbf{q}} + \left[\hat{\mathbf{D}}'_{\mathbf{q}}, \hat{\mathcal{S}}_{\mathbf{q}}\right] = 0. \quad \text{(S46)}$$

The final effective model for the $2 \times 2$ subset of optical branches is thus obtained as:

$$\hat{\mathbf{D}}''_{\text{eff,op}} = \hat{\mathbf{D}}'_{\text{d,op}} + \frac{1}{2}\left[\hat{\eta}^\dagger_{\mathbf{q}}\hat{\mathbf{V}}_{\mathbf{q},\text{op}-\text{ac}} + \hat{\mathbf{V}}^\dagger_{\mathbf{q},\text{op}-\text{ac}}\hat{\eta}_{\mathbf{q}}\right]. \quad \text{(S47)}$$

Note that the derivation here presented does not rely on the hexagonal symmetry and it can be applied as well in case of uniaxial strain. This allows us to determine the parameters $a_0$, $a_1$, $\alpha_0$, $\alpha_1$. Using the values employed in the main text, $\phi_r = 1$, $\phi_t = 0.25$, $M_1 = 1$, $M_2 = 3$ we obtain numerically

$$a_0 = \frac{123}{1600}; \quad a_1 = \frac{9}{320}; \quad \alpha_0 = \frac{3}{2}; \quad \alpha_1 = \frac{3}{20}. \quad \text{(S48)}$$


[S1] L. Zhang and Q. Niu, Phys. Rev. Lett. **115**, 115502 (2015).
[S2] Chen, Hao, Wei Zhang, Qian Niu, and Lifa Zhang, 2D Mater. **6**, 012002 (2018).
[S3] Hidekatsu Suzuura and Tsuneya Ando, Phys. Rev. B 65, 235412 (2002).
[S4] Q. Cai et al., Nanoscale 9,3059 (2017).
[S5] E. Blundo, E. Cappelluti, M. Felici, G. Pettinari, A. Polimeni Applied Physics Reviews 8 (2), 021318 (2021).
